# Supplementary material for: Crossing Numbers of Beyond-Planar Graphs Revisited
Source: arXiv:2105.12452 source file (2021-05-26)

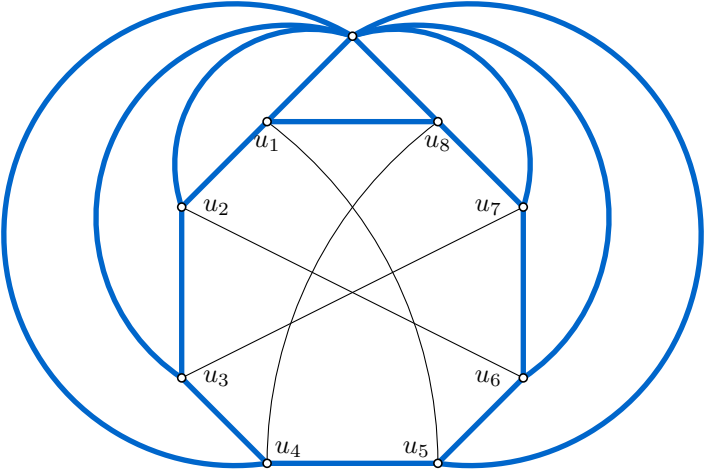

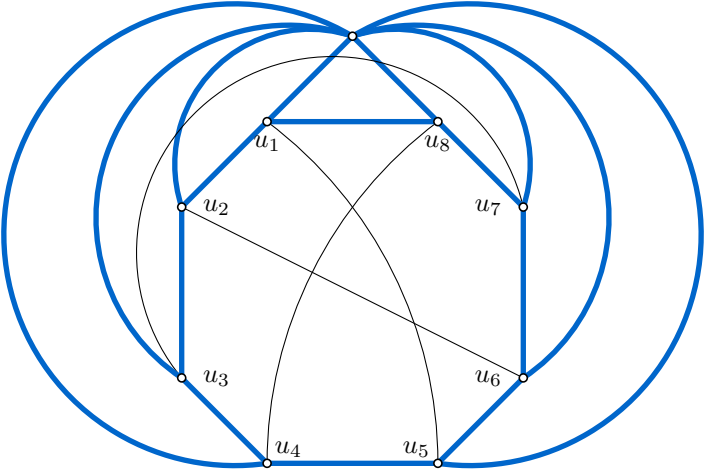

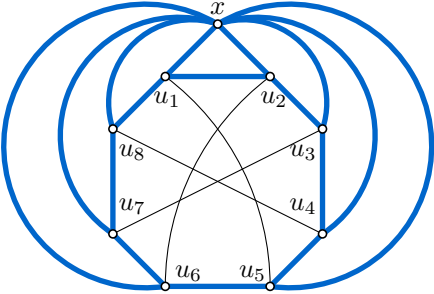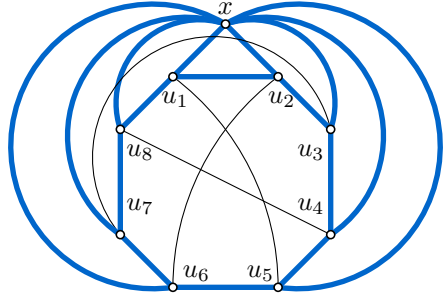

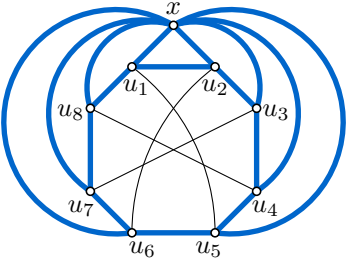

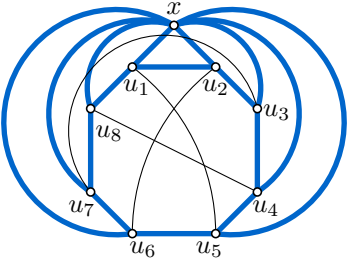

Supplement: Supplementary file 1 [file 1-gap-appendix.pdf]
